# Supplementary material for: Sex and Gender in the Computer Graphics Research Literature
Source: arXiv:2206.00480 ancillary file (2022-06-01)
Supplement: Supplementary file 1 [file supplement.pdf]

# Sex and Gender in the Computer Graphics Research Literature

## Supplemental Material

Ana Dodik<sup>\*†</sup>

MIT  
United States of America

Silvia Sellán<sup>\*</sup>

University of Toronto  
Canada

Theodore Kim

Yale University  
United States of America

Amanda Phillips

Georgetown University  
United States of America

## 1 METHODOLOGY

We reviewed all technical papers published in ACM Transactions on Graphics and presented at either of SIGGRAPH North American or SIGGRAPH Asia between January 2015 and December 2021. We recorded all those which contained explicit mentions of sex or gender and analyzed them from an algorithmic fairness perspective, drawing qualitative and quantitative observations listed below.

## 2 OBSERVATIONS

From a total corpus of 1509, we identified 64 works (see Table 1) that explicitly referenced sex or gender. Studying these in depth, we draw seven global observations relevant to our fairness analysis (see main text), which we detail below. In the inset, we show their aggregate prevalences.

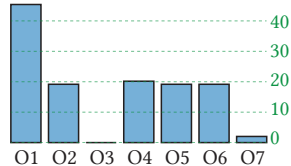

- O1. In 45 (70%) of the reviewed works gender and sex are explicitly presented as binary variables (taking values *male/female* or *man/woman*). None of these 45 mentioned or analyzed the representational bias this choice introduces towards gender non-conforming individuals.
- O2. In 19 (30%) of the reviewed works the nature of the variable is not made explicit (e.g., *we tested our algorithm on images spanning various genders and ethnicities*).
- O3. None of the reviewed works presented gender or sex as non-binary. None of the observed works acknowledged the existence of gender non-conforming, trans, non-binary or intersex individuals.
- O4. In 20 (32%) of the reviewed works gender or sex are used as target or feature binary variables in an algorithm (or suggested to be used as future work). In all these, gender is (implicitly or explicitly) used as a proxy for other variables. What they are a proxy for varies throughout the literature, from body proportions to voice attributes to facial expressions to verbal queues in speech to preferences in attire.
- O5. In 19 (30%) of the reviewed works gender or sex are mentioned as demographic data about the diversity of used datasets. None of the reviewed works explicitly mention the presence of intersex, gender non-conforming, trans or non-binary individuals in their datasets.
- O6. In 19 (30%) of the reviewed works gender or sex are mentioned as demographic data about the diversity of user study participants. Two include participants of “unknown” gender, and none reported participants of non-binary genders.
- O7. 2 (3%) of the reviewed works use or propose new data-based binary gender classifiers to be used on images.

<sup>\*</sup>Joint First Authors

<sup>†</sup>Work done while the author was employed by Meta Platforms, Inc.

Table 1: Recorded SIGGRAPH 2015-2021 technical papers.

| Paper                       | O1 | O2 | O3 | O4 | O5 | O6 | O7 |
|-----------------------------|----|----|----|----|----|----|----|
| [Zhang et al. 2021b]        | X  |    |    |    |    | X  |    |
| [Wu et al. 2021]            |    | X  |    |    |    |    |    |
| [Chen et al. 2021]          | X  |    |    |    | X  |    |    |
| [Sonlu et al. 2021]         | X  |    |    | X  |    |    |    |
| [Wang et al. 2021]          | X  |    |    | X  |    |    |    |
| [Zhang et al. 2021a]        |    | X  |    |    | X  |    |    |
| [Feng et al. 2021]          | X  |    |    |    |    |    |    |
| [Kim and Singh 2021]        | X  |    |    | X  |    |    |    |
| [Wang et al. 2020]          |    | X  |    |    | X  |    |    |
| [Yoon et al. 2020]          | X  |    |    |    | X  | X  |    |
| [Tewari et al. 2020]        |    | X  |    |    |    |    |    |
| [Li et al. 2020]            |    | X  |    |    | X  |    |    |
| [Won et al. 2020]           |    | X  |    |    | X  |    |    |
| [Wisessing et al. 2020]     | X  |    |    | X  |    |    |    |
| [Chen et al. 2020]          | X  |    |    | X  |    |    |    |
| [Riviere et al. 2020]       |    | X  |    |    |    |    |    |
| [Wang et al. 2019]          | X  |    |    | X  |    |    | X  |
| [Yu et al. 2019]            | X  |    |    |    |    | X  |    |
| [Dong et al. 2019]          | X  |    |    |    |    | X  |    |
| [Mueller et al. 2019]       | X  |    |    |    |    | X  |    |
| [Kuo et al. 2019]           |    | X  |    | X  |    |    |    |
| [Sun et al. 2019]           | X  |    |    |    |    |    |    |
| [Cao et al. 2018]           |    | X  |    |    | X  |    |    |
| [Wang et al. 2018a]         | X  |    |    | X  |    |    |    |
| [Geng et al. 2018]          | X  |    |    |    |    | X  |    |
| [Huang et al. 2018]         | X  |    |    |    | X  |    |    |
| [Wang et al. 2018b]         | X  |    |    |    |    | X  |    |
| [Saito et al. 2018]         |    | X  |    |    | X  |    |    |
| [Pai et al. 2018]           | X  |    |    |    | X  |    |    |
| [Zhao et al. 2018]          |    | X  |    |    |    | X  |    |
| [Yang et al. 2018]          | X  |    |    | X  |    |    |    |
| [Zhou et al. 2018]          | X  |    |    |    | X  |    |    |
| [Yamaguchi et al. 2018]     | X  |    |    |    | X  |    |    |
| [Xu et al. 2018]            | X  |    |    |    | X  |    |    |
| [Averbuch-Elor et al. 2017] | X  |    |    |    |    | X  |    |
| [Wen et al. 2017]           |    | X  |    |    |    |    |    |
| [Li et al. 2017]            | X  |    |    | X  |    |    |    |
| [Romero et al. 2017]        | X  |    |    |    | X  |    |    |
| [Mehta et al. 2017]         |    | X  |    |    |    |    |    |
| [Smith and Neff 2017]       | X  |    |    |    | X  |    |    |
| [Durupinar et al. 2016]     | X  |    |    |    | X  |    |    |
| [Koulieris et al. 2017]     | X  |    |    |    |    | X  |    |
| [Konrad et al. 2017]        | X  |    |    |    |    | X  |    |
| [Taylor et al. 2017]        | X  |    |    | X  |    |    |    |
| [Karras et al. 2017]        | X  |    |    | X  |    |    |    |
| [Jin et al. 2017]           | X  |    |    | X  |    |    |    |

**Table 1 continued**

|                               |   |   |  |   |   |   |   |
|-------------------------------|---|---|--|---|---|---|---|
| [Lun et al. 2016]             | X |   |  |   |   | X |   |
| [Olszewski et al. 2016]       | X |   |  |   | X |   |   |
| [Garrido et al. 2016b]        | X |   |  |   |   | X |   |
| [Bartle et al. 2016]          |   | X |  | X | X |   |   |
| [Kemelmacher-Shlizerman 2016] | X |   |  | X |   |   | X |
| [Garrido et al. 2016a]        | X |   |  |   |   |   |   |
| [Edwards et al. 2016]         | X |   |  |   |   | X |   |
| [Selim et al. 2016]           |   | X |  |   |   |   |   |
| [Zell et al. 2015]            | X |   |  |   | X | X |   |
| [Lee et al. 2015]             | X |   |  |   |   | X |   |
| [Adib et al. 2015]            |   | X |  |   |   | X |   |
| [Loper et al. 2015]           | X |   |  | X |   |   |   |
| [Li et al. 2015]              | X |   |  |   |   | X |   |
| [Swedish et al. 2015]         |   | X |  | X |   |   |   |
| [Lun et al. 2015]             | X |   |  |   |   | X |   |
| [Rogge et al. 2014]           | X |   |  | X |   |   |   |
| [Pons-Moll et al. 2015]       | X |   |  | X |   |   |   |

## REFERENCES

- Fadel Adib, Chen-Yu Hsu, Hongzi Mao, Dina Katabi, and Frédo Durand. 2015. Capturing the human figure through a wall. *ACM Transactions on Graphics (TOG)* 34, 6 (2015), 1–13.
- Hadar Averbuch-Elor, Daniel Cohen-Or, Johannes Kopf, and Michael F Cohen. 2017. Bringing portraits to life. *ACM Transactions on Graphics (TOG)* 36, 6 (2017), 1–13.
- Aric Bartle, Alla Sheffer, Vladimir G Kim, Danny M Kaufman, Nicholas Vining, and Floraine Berthouzoz. 2016. Physics-driven pattern adjustment for direct 3D garment editing. *ACM Trans. Graph.* 35, 4 (2016), 50–1.
- Kaidi Cao, Jing Liao, and Lu Yuan. 2018. CariGANs: Unpaired Photo-to-Caricature Translation. *ACM Transactions on Graphics* 37, 6 (2018), 244.
- He Chen, Hoyjoon Park, Kutay Macit, and Ladislav Kavan. 2021. Capturing detailed deformations of moving human bodies. *ACM Transactions on Graphics (TOG)* 40, 4 (2021), 1–18.
- Shu-Yu Chen, Wanchao Su, Lin Gao, Shihong Xia, and Hongbo Fu. 2020. DeepFace-Drawing: Deep generation of face images from sketches. *ACM Transactions on Graphics (TOG)* 39, 4 (2020), 72–1.
- Zhi-Chao Dong, Xiao-Ming Fu, Zeshi Yang, and Ligang Liu. 2019. Redirected smooth mappings for multiuser real walking in virtual reality. *ACM Transactions on Graphics (TOG)* 38, 5 (2019), 1–17.
- Funda Durupinar, Mubbasir Kapadia, Susan Deutsch, Michael Neff, and Norman I Badler. 2016. Perform: Perceptual approach for adding ocean personality to human motion using laban movement analysis. *ACM Transactions on Graphics (TOG)* 36, 1 (2016), 1–16.
- Pif Edwards, Chris Landreth, Eugene Fiume, and Karan Singh. 2016. JALI: an animator-centric viseme model for expressive lip synchronization. *ACM Transactions on graphics (TOG)* 35, 4 (2016), 1–11.
- Yao Feng, Haiwen Feng, Michael J Black, and Timo Bolkart. 2021. Learning an animatable detailed 3D face model from in-the-wild images. *ACM Transactions on Graphics (TOG)* 40, 4 (2021), 1–13.
- Pablo Garrido, Michael Zollhöfer, Dan Casas, Levi Valgaerts, Kiran Varanasi, Patrick Pérez, and Christian Theobalt. 2016a. Reconstruction of personalized 3D face rigs from monocular video. *ACM Transactions on Graphics (TOG)* 35, 3 (2016), 1–15.
- Pablo Garrido, Michael Zollhöfer, Chenglei Wu, Derek Bradley, Patrick Pérez, Thabo Beeler, and Christian Theobalt. 2016b. Corrective 3D reconstruction of lips from monocular video. *ACM Trans. Graph.* 35, 6 (2016), 219–1.
- Jiahao Geng, Tianjia Shao, Youyi Zheng, Yanlin Weng, and Kun Zhou. 2018. Warp-guided gans for single-photo facial animation. *ACM Transactions on Graphics (TOG)* 37, 6 (2018), 1–12.
- Yinghao Huang, Manuel Kaufmann, Emre Aksan, Michael J Black, Otmar Hilliges, and Gerard Pons-Moll. 2018. Deep inertial poser: Learning to reconstruct human pose from sparse inertial measurements in real time. *ACM Transactions on Graphics (TOG)* 37, 6 (2018), 1–15.
- Zeyu Jin, Gautham J Mysore, Stephen Diverdi, Jingwan Lu, and Adam Finkelstein. 2017. Voco: Text-based insertion and replacement in audio narration. *ACM Transactions on Graphics (TOG)* 36, 4 (2017), 1–13.
- Tero Karras, Timo Aila, Samuli Laine, Antti Herva, and Jaakko Lehtinen. 2017. Audio-driven facial animation by joint end-to-end learning of pose and emotion. *ACM Transactions on Graphics (TOG)* 36, 4 (2017), 1–12.
- Ira Kemelmacher-Shlizerman. 2016. Transfiguring portraits. *ACM Transactions on Graphics (TOG)* 35, 4 (2016), 1–8.
- Joonho Kim and Karan Singh. 2021. Optimizing UI layouts for deformable face-rig manipulation. *ACM Transactions on Graphics (TOG)* 40, 4 (2021), 1–12.
- Robert Konrad, Nitish Padmanaban, Keenan Molner, Emily A Cooper, and Gordon Wetzstein. 2017. Accommodation-invariant computational near-eye displays. *ACM Transactions on Graphics (TOG)* 36, 4 (2017), 1–12.
- George-Alex Koulieris, Bee Bui, Martin S Banks, and George Drettakis. 2017. Accommodation and comfort in head-mounted displays. *ACM Transactions on Graphics (TOG)* 36, 4 (2017), 1–11.
- Calvin Kuo, Ziheng Liang, Ye Fan, Jean-Sebastien Blouin, and Dinesh K Pai. 2019. Creating impactful characters: correcting human impact accelerations using high rate IMUs in dynamic activities. *ACM Transactions on Graphics (TOG)* 38, 4 (2019), 1–12.
- Yoonsang Lee, Kyungho Lee, Soon-Sun Kwon, Jiwon Jeong, Carol O’Sullivan, Moon Seok Park, and Jehee Lee. 2015. Push-recovery stability of biped locomotion. *ACM Transactions on Graphics (TOG)* 34, 6 (2015), 1–9.
- Hao Li, Laura Trutoiu, Kyle Olszewski, Lingyu Wei, Tristan Trutna, Pei-Lun Hsieh, Aaron Nicholls, and Chongyang Ma. 2015. Facial performance sensing head-mounted display. *ACM Transactions on Graphics (TOG)* 34, 4 (2015), 1–9.
- Jiaman Li, Zhengfei Kuang, Yajie Zhao, Mingming He, Karl Bladin, and Hao Li. 2020. Dynamic facial asset and rig generation from a single scan. *ACM Trans. Graph.* 39, 6 (2020), 215–1.
- Tianye Li, Timo Bolkart, Michael J Black, Hao Li, and Javier Romero. 2017. Learning a model of facial shape and expression from 4D scans. *ACM Trans. Graph.* 36, 6 (2017), 194–1.
- Matthew Loper, Naureen Mahmood, Javier Romero, Gerard Pons-Moll, and Michael J Black. 2015. SMPL: A skinned multi-person linear model. *ACM transactions on graphics (TOG)* 34, 6 (2015), 1–16.
- Zhaoliang Lun, Evangelos Kalogerakis, and Alla Sheffer. 2015. Elements of style: learning perceptual shape style similarity. *ACM Transactions on graphics (TOG)* 34, 4 (2015), 1–14.
- Zhaoliang Lun, Evangelos Kalogerakis, Rui Wang, and Alla Sheffer. 2016. Functionality preserving shape style transfer. *ACM Transactions on Graphics (TOG)* 35, 6 (2016), 1–14.
- Dushyant Mehta, Srinath Sridhar, Oleksandr Sotnychenko, Helge Rhodin, Mohammad Shafiei, Hans-Peter Seidel, Weipeng Xu, Dan Casas, and Christian Theobalt. 2017. Vnec: Real-time 3d human pose estimation with a single rgb camera. *ACM Transactions on Graphics (TOG)* 36, 4 (2017), 1–14.
- Franziska Mueller, Micah Davis, Florian Bernard, Oleksandr Sotnychenko, Mickael Verschoor, Miguel A Otaduy, Dan Casas, and Christian Theobalt. 2019. Real-time pose and shape reconstruction of two interacting hands with a single depth camera. *ACM Transactions on Graphics (TOG)* 38, 4 (2019), 1–13.
- Kyle Olszewski, Joseph J Lim, Shunsuke Saito, and Hao Li. 2016. High-fidelity facial and speech animation for VR HMDs. *ACM Transactions on Graphics (TOG)* 35, 6 (2016), 1–14.
- Dinesh K Pai, Austin Rothwell, Pearson Wyder-Hodge, Alistair Wick, Ye Fan, Egor Larionov, Darcy Harrison, Debanga Raj Neog, and Cole Shing. 2018. The human touch: Measuring contact with real human soft tissues. *ACM Transactions on Graphics (TOG)* 37, 4 (2018), 1–12.
- Gerard Pons-Moll, Javier Romero, Naureen Mahmood, and Michael J Black. 2015. Dyna: A model of dynamic human shape in motion. *ACM Transactions on Graphics (TOG)* 34, 4 (2015), 1–14.
- Jérémy Riviere, Paulo Gotardo, Derek Bradley, Abhijeet Ghosh, and Thabo Beeler. 2020. Single-shot high-quality facial geometry and skin appearance capture. (2020).
- Lorenz Rogge, Felix Klose, Michael Stengel, Martin Eisemann, and Marcus Magnor. 2014. Garment replacement in monocular video sequences. *ACM Transactions on Graphics (TOG)* 34, 1 (2014), 1–10.
- Javier Romero, Dimitris Tzionas, and Michael J Black. 2017. Embodied Hands: Modeling and Capturing Hands and Bodies Together. *ACM Transactions on Graphics* 36, 6 (2017).
- Shunsuke Saito, Liwen Hu, Chongyang Ma, Hikaru Ibayashi, Jinjie Luo, and Hao Li. 2018. 3D hair synthesis using volumetric variational autoencoders. *ACM Transactions on Graphics (TOG)* 37, 6 (2018), 1–12.
- Ahmed Selim, Mohamed Elgharib, and Linda Doyle. 2016. Painting style transfer for head portraits using convolutional neural networks. *ACM Transactions on Graphics (ToG)* 35, 4 (2016), 1–18.
- Harrison Jesse Smith and Michael Neff. 2017. Understanding the impact of animated gesture performance on personality perceptions. *ACM Transactions on Graphics (TOG)* 36, 4 (2017), 1–12.
- Sinan Sonlu, Ugur Gudukbay, and Funda Durupinar. 2021. A conversational agent framework with multi-modal personality expression. *ACM Transactions on Graphics (TOG)* 40, 1 (2021), 1–16.
- Tiancheng Sun, Jonathan T Barron, Yun-Ta Tsai, Zexiang Xu, Xueming Yu, Graham Fyfe, Christoph Rhemann, Jay Busch, Paul E Debevec, and Ravi Ramamoorthi. 2019. Single image portrait relighting. *ACM Trans. Graph.* 38, 4 (2019), 79–1.
- Tristan Swedish, Karin Roesch, Ik-Hyun Lee, Krishna Rastogi, Shoshana Bernstein, and Ramesh Raskar. 2015. EyeSelfie: self directed eye alignment using reciprocal

## Supplemental Material

- eye box imaging. *ACM Transactions on Graphics (TOG)* 34, 4 (2015), 1–10.
- Sarah Taylor, Taehwan Kim, Yisong Yue, Moshe Mahler, James Krahe, Anastasio Garcia Rodriguez, Jessica Hodgins, and Iain Matthews. 2017. A deep learning approach for generalized speech animation. *ACM Transactions on Graphics (TOG)* 36, 4 (2017), 1–11.
- Ayush Tewari, Mohamed Elgharib, Florian Bernard, Hans-Peter Seidel, Patrick Pérez, Michael Zollhöfer, and Christian Theobalt. 2020. Pie: Portrait image embedding for semantic control. *ACM Transactions on Graphics (TOG)* 39, 6 (2020), 1–14.
- Jiayi Wang, Franziska Mueller, Florian Bernard, Suzanne Sorli, Oleksandr Sotnychenko, Neng Qian, Miguel A Otaduy, Dan Casas, and Christian Theobalt. 2020. Rgb2hands: real-time tracking of 3d hand interactions from monocular rgb video. *ACM Transactions on Graphics (ToG)* 39, 6 (2020), 1–16.
- Tuanfeng Y Wang, Duygu Ceylan, Jovan Popovic, and Niloy J Mitra. 2018a. Learning a shared shape space for multimodal garment design. *arXiv preprint arXiv:1806.11335* (2018).
- Xi Wang, Sebastian Koch, Kenneth Holmqvist, and Marc Alexa. 2018b. Tracking the gaze on objects in 3D: How do people really look at the bunny? *ACM Transactions on Graphics (TOG)* 37, 6 (2018), 1–18.
- Yupan Wang, Guiqing Li, Huiqian Zhang, Xinyi Zou, Yuxin Liu, and Yongwei Nie. 2021. PanoMan: Sparse Localized Components–based Model for Full Human Motions. *ACM Transactions on Graphics (TOG)* 40, 2 (2021), 1–17.
- Yujia Wang, Wenguan Wang, Wei Liang, and Lap-Fai Yu. 2019. Comic-guided speech synthesis. *ACM Transactions on Graphics (TOG)* 38, 6 (2019), 1–14.
- Quan Wen, Feng Xu, Ming Lu, and Jun-Hai Yong. 2017. Real-time 3D eyelids tracking from semantic edges. *ACM Transactions on Graphics (TOG)* 36, 6 (2017), 1–11.
- Pisut Wisessing, Katja Zibrek, Douglas W Cunningham, John Dingliana, and Rachel McDonnell. 2020. Enlighten me: Importance of brightness and shadow for character emotion and appeal. *ACM Transactions on Graphics (TOG)* 39, 3 (2020), 1–12.
- Jungdam Won, Deepak Gopinath, and Jessica Hodgins. 2020. A scalable approach to control diverse behaviors for physically simulated characters. *ACM Transactions on Graphics (TOG)* 39, 4 (2020), 33–1.
- Yiqian Wu, Yong-Liang Yang, Qinjie Xiao, and Xiaogang Jin. 2021. Coarse-to-fine: facial structure editing of portrait images via latent space classifications. *ACM Transactions on Graphics (TOG)* 40, 4 (2021), 1–13.
- Weipeng Xu, Avishek Chatterjee, Michael Zollhöfer, Helge Rhodin, Dushyant Mehta, Hans-Peter Seidel, and Christian Theobalt. 2018. Monoperfcap: Human performance capture from monocular video. *ACM Transactions on Graphics (ToG)* 37, 2 (2018), 1–15.
- Shugo Yamaguchi, Shunsuke Saito, Koki Nagano, Yajie Zhao, Weikai Chen, Kyle Olaszewski, Shigeo Morishima, and Hao Li. 2018. High-fidelity facial reflectance and geometry inference from an unconstrained image. *ACM Transactions on Graphics (TOG)* 37, 4 (2018), 1–14.
- Shan Yang, Zherong Pan, Tanya Amert, Ke Wang, Licheng Yu, Tamara Berg, and Ming C Lin. 2018. Physics-inspired garment recovery from a single-view image. *ACM Transactions on Graphics (TOG)* 37, 5 (2018), 1–14.
- Youngwoo Yoon, Bok Cha, Joo-Haeng Lee, Minsu Jang, Jaeyeon Lee, Jaehong Kim, and Geehyuk Lee. 2020. Speech gesture generation from the trimodal context of text, audio, and speaker identity. *ACM Transactions on Graphics (TOG)* 39, 6 (2020), 1–16.
- Difeng Yu, Hai-Ning Liang, Xueshi Lu, Kaixuan Fan, and Barrett Ens. 2019. Modeling endpoint distribution of pointing selection tasks in virtual reality environments. *ACM Transactions on Graphics (TOG)* 38, 6 (2019), 1–13.
- Eduard Zell, Carlos Aliaga, Adrian Jarabo, Katja Zibrek, Diego Gutierrez, Rachel McDonnell, and Mario Botsch. 2015. To stylize or not to stylize? The effect of shape and material stylization on the perception of computer-generated faces. *ACM Transactions on Graphics (TOG)* 34, 6 (2015), 1–12.
- Haotian Zhang, Cristobal Sciuotto, Maneesh Agrawala, and Kayvon Fatahalian. 2021a. Vid2player: Controllable video sprites that behave and appear like professional tennis players. *ACM Transactions on Graphics (TOG)* 40, 3 (2021), 1–16.
- Hao Zhang, Yuxiao Zhou, Yifei Tian, Jun-Hai Yong, and Feng Xu. 2021b. Single Depth View Based Real-Time Reconstruction of Hand-Object Interactions. *ACM Transactions on Graphics (TOG)* 40, 3 (2021), 1–12.
- Nanxuan Zhao, Ying Cao, and Rynson WH Lau. 2018. What characterizes personalities of graphic designs? *ACM Transactions on Graphics (TOG)* 37, 4 (2018), 1–15.
- Yang Zhou, Zhan Xu, Chris Landreth, Evangelos Kalogerakis, Subhansu Maji, and Karan Singh. 2018. Visemenet: Audio-driven animator-centric speech animation. *ACM Transactions on Graphics (TOG)* 37, 4 (2018), 1–10.
